# Supplementary material for: Securing Behavior-based Opinion Spam Detection
Source: arXiv:1811.03739 source file (2018-11-09)
Supplement: Supplementary file 1 [file appendix.tex]

\appendix
\section*{Appendix}
\small
\subsection{Derivation $\hat{x}_{t+1}(\delta)$}
\label{sec:app_1}
Define the $d$ dimensional perturbation vector $\boldsymbol{\delta}=[0,\dots, 0,\delta]^{\top}$ as an attack to poison $\mathbf{x}_{t-d+1}^{t}$,
\begin{eqnarray}
\begin{aligned}
\hat{x}_{t+1}(\delta) &= \tilde{\boldsymbol{\theta}}^{(t+1)\top} \tilde{\mathbf{x}}_{t-d+1}^{t} \nonumber \\
&= (\boldsymbol{\theta}^{(t)} + \eta (x_{t} + \delta - \hat{x}_{t}) \mathbf{x}_{t-d}^{t-1})^{\top} (\mathbf{x}_{t-d+1}^{t} + \boldsymbol{\delta})\nonumber\\
&= (\boldsymbol{\theta}^{(t)} + \eta (x_t - \hat{x}_t)\mathbf{x}_{t-d}^{t-1} + \eta \delta \mathbf{x}_{t-d}^{t-1})^{\top}(\mathbf{x}_{t-d+1}^{t} + \boldsymbol{\delta})\\
\end{aligned}
\end{eqnarray}
$\boldsymbol{\theta}^{(t)}+\eta (x_t - \hat{x}_t) \mathbf{x}_{t-d}^{t-1}$ is $\boldsymbol{\theta}^{(t+1)}$,
the AR model if there were no attack.
The above can be written as
\begin{eqnarray}
\begin{aligned}
\hat{x}_{t+1}(\delta)
=& \boldsymbol{\theta}^{(t+1)\top} \mathbf{x}_{t-d+1}^{t} + \boldsymbol{\theta}^{(t+1)\top}\boldsymbol{\delta} \\
&+ \eta \delta ((\mathbf{x}_{t-d}^{t-1})^{\top} \mathbf{x}_{t-d+1}^{t}) + \eta \delta ((\mathbf{x}_{t-d}^{t-1})^{\top}\boldsymbol{\delta}) \nonumber\\
=& \hat{x}_{t+1} + [\theta^{(t+1)}_{1} + \eta ((\mathbf{x}_{t-d}^{t-1})^{\top} \mathbf{x}_{t-d+1}^{t})]\delta + \eta \delta^2 {x}_{t-1}\nonumber
\end{aligned}
\end{eqnarray}

\subsection{Derivation of the Lagrangian of Eq.~\ref{eq:kl_primal}}
\label{sec:app_2}
\begin{equation}
\begin{split}
    L(p,\alpha,\beta,\lambda,\gamma,\mu) &= \sum_ip_i\log{\frac{p_i}{\bar{p}_i}}+\alpha(\sum_iip_i-U) \\ &+\beta(-\sum_iip_i+B)+\lambda(\sum_i\mathbb{I}(i)p_i-P)\\&+\gamma(\sum_ip_i\log{p_i}+H)+\mu(\sum_ip_i-1)
\end{split}
\end{equation}
\begin{equation}
\mathbb{I}(i)=
\begin{cases}
0 &i=1,2,3 \\
1 &i=4,5
\end{cases}
\end{equation}
where $\alpha$, $\beta$, $\lambda$, $\gamma$, $\mu$ are Lagrangian multipliers for the five constraints, respectively. Take the derivative of $L$ with respect to $p_i$, we have
\begin{equation}
\frac{\partial{L}}{\partial{p_i}}=
1+\log{\frac{p_i}{\bar{p}_i}}+(\alpha-\beta)i+\lambda\mathbb{I}(i)+\gamma(1+\log{p_i})+\mu 
\end{equation}
Equate the derivative to 0 and solve for $p_i$, we have
\begin{equation}
p_i=
\exp\left\{\frac{\log{\bar{p}_i}-(\alpha-\beta)i-1-\lambda\mathbb{I}(i)-\gamma-\mu}{1+\gamma}\right\} = \exp\left(\frac{S_i-\mu}{1+\gamma}\right)
\end{equation}
where $S_i=\log{\bar{p}_i}-(\alpha-\beta)i-1 - \lambda\mathbb{I}(i)-\gamma$.
Since $\sum_i p_i=1$,
$\exp\left(\frac{\mu}{1+\gamma}\right)=\sum_i
\exp\left(\frac{S_i}{1+\gamma}\right)=Z$ is the normalizer.
Plug this $p_i$ back into $L$, we have the Lagrangian
\begin{equation}
L(\alpha, \beta, \lambda, \gamma)=-(1+\gamma)\log{Z}-(1+\gamma)-\alpha U+\beta B-\lambda p+\gamma H
\end{equation}
which lower bounds the optimal value of the primal problem Eq.~(\ref{eq:kl_primal}).
Since the primal is convex, we have strong duality and the maximum of the dual function is exactly the minimum of the primal function.
To this end, we solve the following Lagrange dual problem:
\begin{equation}
\begin{aligned}
& \underset{\alpha,\beta,\gamma,\lambda}{\max} 
& & L(\alpha,\beta,\gamma,\lambda) \\
& \text{subject to}
& & \alpha \geq 0, \beta \geq 0, \gamma \geq 0, \lambda \geq 0
\end{aligned}
\end{equation}

\begin{equation}
    \frac{\partial{L}}{\partial{\alpha}}
    = -\frac{1+\gamma}{Z}\frac{\partial{Z}}{\partial{\alpha}}-U
\end{equation}
\begin{equation}
\frac{\partial{Z}}{\partial{\alpha}}=\frac{\partial}{\partial{\alpha}}\sum_i\exp\left(\frac{S_i}{1+\gamma}\right)
=\frac{1}{1+\gamma}\sum_i\exp\left(\frac{S_i}{1+\gamma}\right)\frac{\partial{S_i}}{\partial{\alpha}}
\end{equation}
Plug the above equation into Eq. (9), we have
\begin{equation}
\begin{split}
\frac{\partial{L}}{\partial{\alpha}}
&=-\frac{1+\gamma}{Z}\frac{1}{1+\gamma}\sum_i\exp\left(\frac{S_i}{1+\gamma}\right)\frac{\partial{S_i}}{\partial{\alpha}}-U \\
&=-\sum_i\frac{\exp{(S_i/(1+\gamma))}}{Z}\frac{\partial{S_i}}{\partial{\alpha}}-U\\
%&=-\sum_ip_i\frac{\partial{S_i}}{\partial{\alpha}}-U\\
&=\sum_i p_i i -U
\end{split}
\end{equation}
%The last equation is due to $\partial{S_i}/\partial{\alpha}=-i$
Similarly,
%\begin{equation}
%    \frac{\partial{L}}{\partial{\beta}}
%    = -\frac{1+\gamma}{Z}\frac{\partial{Z}}{\partial{\beta}}-(1+\gamma)\sum_i\frac{\partial{p_i}}{\partial{\beta}}+B
%\end{equation}
%\begin{equation}
%\frac{\partial{Z}}{\partial{\beta}}=\frac{\partial}{\partial{\beta}}\sum_i\text{exp}\frac{S_i}{1+\gamma}=\frac{1}{1+\gamma}\sum_i\text{exp}(\frac{S_i}{1+\gamma})\frac{\partial{S_i}}{\partial{\beta}}
%\end{equation}
%Plug the above equation into Eq. (12), we have
\begin{equation}
%\begin{split}
\frac{\partial{L}}{\partial{\beta}}
%&=-\sum_ip_i\frac{\partial{S_i}}{\partial{\beta}}+B \\
=-\sum_i p_i i+B 
%\end{split}
\end{equation}
%The last equation is due to $\partial{S_i}/\partial{\beta}=i$
%\begin{equation}
%    \frac{\partial{L}}{\partial{\lambda}}
%    = -\frac{1+\gamma}{Z}\frac{\partial{Z}}{\partial{\lambda}}-(1+\gamma)\sum_i\frac{\partial{p_i}}{\partial{\lambda}}-P
%\end{equation}
%\begin{equation}
%\frac{\partial{Z}}{\partial{\lambda}}=\frac{\partial}{\partial{\lambda}}\sum_i\text{exp}\frac{S_i}{1+\gamma}=\frac{1}{1+\gamma}\sum_i\text{exp}(\frac{S_i}{1+\gamma})\frac{\partial{S_i}}{\partial{\lambda}}
%\end{equation}
%Plug the above equation into Eq. (15), we have
\begin{equation}
%\begin{split}
    \frac{\partial{L}}{\partial{\lambda}}
%    &=-\sum_ip_i\frac{\partial{S_i}}{\partial{\lambda}}-P \\
    =\sum_ip_i\mathbb{I}(i)-P
%\end{split}
\end{equation}
%The last equation is due to $\partial{S_i}/\partial{\lambda}=-\mathbbm{1}(i)$
%\begin{equation}
%    \frac{\partial{L}}{\partial{\gamma}}
%    = -\log Z-\frac{1+\gamma}{Z}\frac{\partial{Z}}{\partial{\gamma}}-\sum_ip_i-(1+\gamma)\sum_i\frac{\partial{p_i}}{\partial{\gamma}}+H
%\end{equation}
%\begin{equation}
%\frac{\partial{Z}}{\partial{\gamma}}=\frac{1}{1+\gamma}\sum_i\text{exp}(\frac{S_i}{1+\gamma})\left(\frac{\partial{S_i}}{\partial{\gamma}}-\frac{S_i}{1+\gamma}\right)
%\end{equation}
%Plug the above equation into Eq. (18), we have
\begin{equation}
%\begin{split}
\frac{\partial{L}}{\partial{\gamma}}
%&=-\log Z-\sum_ip_i\left(\frac{\partial{S_i}}{\partial{\gamma}}-\frac{S_i}{1+\gamma}\right)+H \\
=-\sum_ip_i\left(-1-\frac{S_i}{1+\gamma}\right)
-\log Z
+H-1
%\end{split}
\end{equation}
%The last equation is due to $\partial{S_i}/\partial{\gamma}=-1$
